# Supplementary material for: Stratified Prediction-Powered Inference for Hybrid Language Model Evaluation
Source: arXiv:2406.04291 source file (2024-12-03)
Supplement: Supplementary file 1 [file 07_appendix.tex]

\section{Experimental Details}

\subsection{Python Implementation}  \label{sec:python}

\begin{table}
\begin{small}
\begin{verbatim}
import diem
def theta_fn(data):
  # pandas DataFrames holding S_n and S_N
  labeled_df, unlabeled_df = data
  return {
    'autorater_mean':
      diem.Mean(unlabeled_df.f),
    'rectifier':
      diem.Mean(labeled_df.y - labeled_df.f)
  }
def g_fn(autorater_mean, rectifier_mean):
  return autorater_mean + rectifier_mean
lo, hi = diem.MCIScorer(
  data, theta_fn, g_fn).score().ci()
\end{verbatim}
\end{small}
\caption{Sample Python code that implements the difference estimate.}  \label{tab:python}
\end{table}

Table~\ref{tab:python} illustrates an implementation of Monte Carlo integration in our software package, called \verb|diem| (for Design of Interval Estimation Methods). 
Implementing a PPI method is broken down into two steps: constructing and naming the $\theta$'s (means and proportions) that will be used in $g$, and then a Python implementation of the proxy estimand.  The \verb|Mean| object is 
responsible for sampling from the posterior, and the \verb|Scorer| object orchestrates sampling from each posterior, passing the samples to the proxy estimate function (here \verb|g_fn|), and creating an object to hold the results.

The code allows one to construct only three kinds of parameter posteriors, called \verb|Mean| (which has a Gaussian posterior for $n > 30$), \verb|Proportion| (a Beta posterior, using a Jeffrey's prior), and \verb|KProportion| (a Dirichlet posterior, for which we use the prior $\alpha_1=\ldots\alpha_K = \frac{1}{K}$.).
For \verb|Mean|s the Gaussian has a variance of $\hat{\sigma}^2/n$ where $\hat{\sigma}^2$ is the sample variance.  Instead of a Gaussian we use the appropriate Student's $T$ curve for $n<30$, which reflects standard classical statistical practice.

\subsection{Experiments: Seahorse and Attributed QA} \label{app:seahorse}

Regression trees were fit using the \verb|DecisionTreeRegressor| implementation from the \verb|sklearn.tree| package,
using the \verb|max_leaf_nodes| parameter to fix $K$.  
When tuning $K$, we considered the values
$2, 3, 5, 10, 20, 40$ and picked the one with smallest CI width.

The equal-frequency partitions were always selected using only the unlabeled data, and the tree is fit using only the labeled data.  This means that it is possible for there to be very few members of a partition in $S_n$ (for equal-frequency partitions) or $\twid{S}_N$ for tree partitions.  To fix this, we used a simple post-processing step, where (1) if there are any partitions that have fewer than 3 members in either $S_n$ or $\twid{S}_N$, those partitions are deleted, and replaced with a special ``miscellaneous'' partition and then (2) if the ``miscellaneous'' partition has fewer than 3 members in either part of the data, the smallest partition is deleted and its members are added to the ``miscellaneous'' one.

\begin{figure}[tb]
    \includegraphics[width=0.45\textwidth]{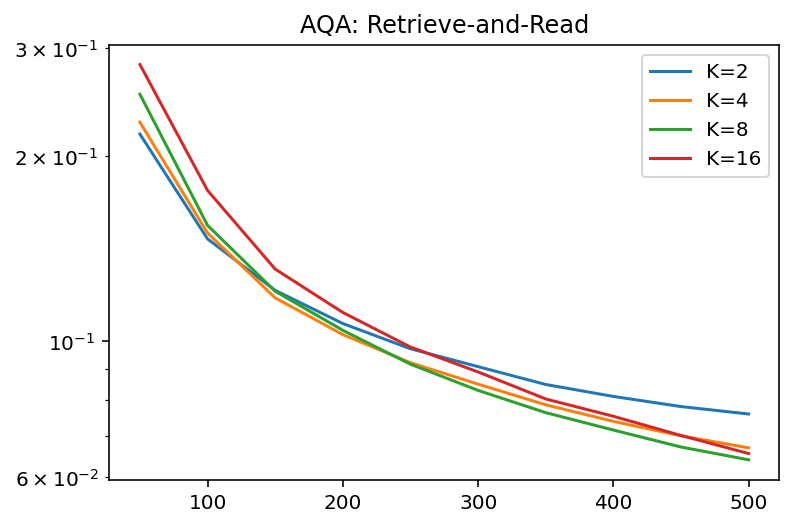}
\caption{Varying the number of partitions for one dataset.}
\label{fig:vary-part-k}
\end{figure}

In Figure~\ref{fig:vary-part-k} we vary the number of partitions for a single dataset (note the $y$-axis here is log scale, to make it easier to separate the results).  In general the best results are to use few partitions for small $n$, and more with larger $n$.

\subsection{Synthetic Data} \label{sec:kamaloo-coverage}

To generate synthetic data similar to the data of \cite{kamalloo-etal-2023-evaluating}
we used this procedure.
\begin{enumerate}
\item We created a Beta posterior distributions for $p(H|A)$, $p(H|\neg A)$, and $p(A)$ for each QA method at $n=300$.
\item To create a set of ``true'' values $\theta^*$ , we pick a QA method uniformly, and then sample values from the corresponding Betas.  This maintains dependencies that might exist in the parameter values, but also allows many different ``true'' $\theta^*$'s to be chosen.
\item Finally, we uniformly sample values of $n \sim \{100,\ldots,500\}$ and $N \sim \{3000,\ldots,4000\}$, and then generate a synthetic dataset of the right size using the ``true'' $\theta^*$ sampled in step 2.  
\end{enumerate}

We then run the chain rule estimate on these generated datasets and test for coverage.

For the experiments of Section~\ref{sec:aqa-coverage}, we used the same procedure, except instead starting with Beta distributions at $n=300$, we consider each $n$ used in creating the curves of Figure~\ref{fig:pairs} (i.e., $n=30, 50, 100, \ldots 300, 400, \ldots, 1000$) for a total of 826 different Betas.  To create true $\theta^*$ values, we uniformly sample $n \sim \{500, \ldots, 1000\}$ and $N \sim \{2000,4000\}$. 

\subsection{Linearizing the choices made by the abstaining autorater} \label{sec:linear}

\begin{table}
\centering
\begin{tabular}{lcl}
\toprule
            & mean interval & width ratio\\
            & width         & to classical\\
\midrule
~~chain rule estimate & 0.088 & 0.84 \\
~~difference estimate & 0.149 & 1.43\\
~~classical   & 0.104 & 1.00 \\
\midrule
\textit{$n=-1, y=+1, u=0$} &  & \\
~~difference estimate & 0.193 & 0.92 \\
~~classical   & 0.210 & 1.00 \\
\bottomrule
\end{tabular}
\caption{Alternative linearization schemes for abstaining autoraters.}
\label{tab:linearize}
\end{table}

The discrete values ``n'', ``y'', and ``u'' were internally encoded by the Dirichlet as integers 0, 1, and 2 respectively.  In addition to the scheme described in the paper, we considered several other linearization schemes, all of which were dramatically worse for the difference estimate, as summarized in Table~\ref{tab:linearize}.

We considered all six permutations of these codes and report numbers for the best in the top of the table.   It is a little surprising that the difference estimate is so much worse here worse than the classical estimate.  In our experiments we did note that the difference estimate does give an improvement over the classical method when you map $n$ to $-1$, $y$ to $+1$, and $u$ to $0$, but in this case all the CI widths are larger.
